# Supplementary material for: Low temperature synthesis of heterostructures of transition metal dichalcogenide alloys (WxMo1-xS2) and graphene with superior catalytic performance for hydrogen evolution
Source: arXiv:1703.08597 source file (2017-05-05)
Supplement: Supplementary file 1 [file rGO_XS2_SI_20170501.pdf]

## Supporting Information

# Low Temperature Synthesis of Heterostructures of Transition Metal Dichalcogenide Alloys ( $W_xMo_{1-x}S_2$ ) and Graphene with Superior Catalytic Performance for Hydrogen Evolution

*Yu Lei<sup>1†</sup>, Srimanta Pakhira<sup>2,3,4,5†</sup>, Kazunori Fujisawa<sup>6</sup>, Xuyang Wang<sup>7</sup>, Oluwagbenga Oare Iyiola<sup>2,3,4,5</sup>, Néstor Perea López<sup>6,8</sup>, Ana Laura Elías<sup>6,8</sup>, Lakshmy Pulickal Rajukumar<sup>1,8</sup>, Chanjing Zhou<sup>1</sup>, Bernd Kabius<sup>1</sup>, Nasim Alem<sup>1</sup>, Morinobu Endo<sup>9</sup>, Ruitao Lv<sup>7\*</sup>, Jose L. Mendoza-Cortes<sup>2,3,4,5\*</sup>, and Mauricio Terrones<sup>1,6,8,9,10\*</sup>*

<sup>1</sup>Department of Materials Science and Engineering & Materials Research Institute, The Pennsylvania State University, University Park, Pennsylvania 16802, United States;

<sup>2</sup>Department of Chemical & Biomedical Engineering, FAMU-FSU College of Engineering, Florida State University (FSU), Tallahassee, Florida, 32310, United States; <sup>3</sup>Department of Scientific Computing, 400 Dirac Science Library, FSU, Tallahassee, Florida, 32304, United States; <sup>4</sup>Materials Science and Engineering Program, High Performance Materials Institute; FSU, Tallahassee, Florida, 32310; <sup>5</sup>Condensed Matter Theory, National High Magnetic Field Laboratory (NHMFL), FSU, Tallahassee, Florida, 32310, United States; <sup>6</sup>Department of Physics, The Pennsylvania State University, University Park, Pennsylvania 16802, United

States; <sup>7</sup>Key Laboratory of Advanced Materials (MOE), School of Materials Science and Engineering, Tsinghua University, Beijing, 100084, China; <sup>8</sup>Center for 2-Dimensional and Layered Materials, The Pennsylvania State University, University Park, Pennsylvania 16802, United States; <sup>9</sup>Institute of Carbon Science and Technology, Shinshu University, Wakasato 4-17-1, Nagano, 380-8553, Japan; and <sup>10</sup>Department of Chemistry, The Pennsylvania State University, University Park, Pennsylvania 16802, United States. †The authors Y.L. and S.P. contributed equally in this article. Correspondence and requests for materials should be addressed to R.L, J.L.M-C. or M.T. (email: lvruitao@tsinghua.edu.cn, jmendozacortes@fsu.edu, or mut11@psu.edu).

## Characterization

The scanning electron microscopy (SEM) was carried out using a FEI Nova NanoSEM 630 FESEM equipped with an energy dispersive spectroscopy (EDS).

Raman spectroscopy and mapping were performed in a Renishaw inVia confocal microscope-based Raman spectrometer with a spectral resolution better than  $2\text{ cm}^{-1}$ . We used a 514.5 nm laser excitation, and the  $520.5\text{ cm}^{-1}$  phonon mode from the silicon substrate was used for calibration.

X-ray photoelectron spectroscopy (XPS) experiments were performed using a Physical Electronics VersaProbe II instrument equipped with a monochromatic Al  $K\alpha$  x-ray source ( $h\nu = 1486.7\text{ eV}$ ) and a concentric hemispherical analyzer. Charge neutralization was performed using both low energy electrons ( $<5\text{ eV}$ ) and argon ions. The binding energy axis was calibrated using sputter cleaned Cu foil (Cu  $2p_{3/2} = 932.7\text{ eV}$ , Cu  $2p_{3/2} = 75.1\text{ eV}$ ). Peaks were charge referenced to C-C band in the carbon 1s spectra at 284.4 eV. Measurements were made at a takeoff angle of  $45^\circ$  with respect to the sample surface plane. This resulted in a typical sampling depth of 3-6 nm (95% of the signal originated from this depth or shallower). Quantification was done using instrumental relative sensitivity factors (RSFs) that account for the X-ray cross section and inelastic mean free path of the electrons. These were derived from fresh exfoliated reference  $\text{WS}_2$  and  $\text{MoS}_2$  samples from HQ Graphene.

The rGO/ $\text{WS}_2$  and rGO/ $\text{MoS}_2$  films with similar dendritic-like morphology were formed, as shown in the SEM images (Figure S4a, d). EDS mappings in Figure S4b-c indicate that tungsten and sulfur were mostly detected on the dendritic-branches with the  $\text{WS}_2$  stoichiometry, as well as  $\text{MoS}_2$  (Figure S4e-f).

We prepared four different samples from precursor solution with different GO and ATTT weight ratios to investigate the role of GO working as surfactant in the formation of WS<sub>2</sub>. Raman was used to study the structure of the synthetic samples (Figure S5a). It has been reported that under 514.5 nm laser excitation, the longitudinal acoustic mode  $2LA(M)$  (*ca.* 352 cm<sup>-1</sup>) of WS<sub>2</sub> monolayers has a remarkable increase in intensity due to an active double resonance process, which causes that the intensity ratio of  $2LA(M)$  to  $A_{1g}$  ( $I_{2LA}/I_{A1g}$ ) almost reach 2.2 in monolayer as shown in Figure S5b.<sup>1</sup> As layer number increases to 3 layers, this intensity ratio ( $I_{2LA}/I_{A1g}$ ) decreases to *ca.* 0.7.<sup>1</sup> It can be seen that the intensity ratio of  $I_{2LA}/I_{A1g}$  increases with the reduction of ATTT in the precursor solution (see Figure S5c). The highest intensity ratio of  $I_{2LA}/I_{A1g}$  obtained is *ca.* 1.33 when ATTT amount is the lowest (ATTT: GO=1:2). When ATTT amount increases 10 times (ATTT: GO=5:1), the intensity ratio of  $I_{2LA}/I_{A1g}$  is *ca.* 1.00 (see Figure S5a, c). In general, this ratio ( $I_{2LA}/I_{A1g}$ ) is always below 1.00 for WS<sub>2</sub> with a layer number exceeding 3 (see Figure S5b).<sup>1</sup> The obtained intensity ratio  $I_{2LA}/I_{A1g}$  ranging from 1.00 to 1.33 suggests the presence of monolayers and bilayers of WS<sub>2</sub>, exposing more catalytic active surface area when compared to the bulk structure. However, since low ATTT amounts result in smaller WS<sub>2</sub> coverage, the sample prepared with ATTT: GO=1:1 has the optimal WS<sub>2</sub> coverage and the optimal  $I_{2LA}/I_{A1g}$  ratio, which is about 1.27. This material was used for further structural characterization and catalytic HER.

To further investigate the distribution of WS<sub>2</sub> layer numbers within the film, a Raman mapping using the 514.5 nm laser excitation was recorded (Figure S6). The optical image shown in Figure S6a displays the similar dendritic-like morphology as the SEM image (Figure S4a). It is noteworthy that the intensity ratio of  $2LA(M)$  to  $A_{1g}$  is equal to or higher than 1 across

the film, especially the WS<sub>2</sub> accumulated dendritic-branches on which the ratio is *ca.* 1.4 (Figure S6d), indicating that fewer layers WS<sub>2</sub> was formed across the film.

After transferring the films onto TEM grids, vertically aligned heterostructures of rGO/WS<sub>2</sub> was found from the dendritic area (Figure S7a). Discontinuous laminar structures constructed from mono- (Figure S7b) and few-layered (Figure S7c) WS<sub>2</sub> with rGO layers were found in the vertically aligned rGO/WS<sub>2</sub> by HRTEM. The intensity line profiles indicate that few-layer WS<sub>2</sub> with ~0.68 nm interlayer spacing is sandwiched with rGO layers exhibiting ~0.33 nm interlayer spacing, as well as monolayer WS<sub>2</sub> within the rGO layers.

High-resolution transmission electron microscopy (HRTEM) observations were performed in a JEM-2010F (JEOL) equipped with a field emission electron source and an ultrahigh resolution pole piece (*Cs* = 0.5 nm). An accelerating voltage at 200 kV was used for imaging.

The scanning transmission electron microscopy (STEM) observation was carried out by FEI Titan<sup>3</sup> G2 S/TEM operated at 80 keV and the high-angle annular dark field (HAADF) detector was used for Z-contrast imaging.

### **Theoretical DFT Calculations (thermodynamics and kinetics): The Chemical Reaction Mechanism on W<sub>x</sub>Mo<sub>1-x</sub>S<sub>2</sub>.**

The Tafel slope *b* can be expressed by the mathematical expression  $b = 2.3RT/nF$ ; where *R* is the universal gas constant (8.314458 J K<sup>-1</sup> mol<sup>-1</sup>), *F* is the Faraday constant (96485.33289), and *n* is the difference between in the number of electrons between the ground state and the transition state. In the present HER reaction, *n* = 1 since the ground state has been shifted to the negatively charged structure as shown in Figure S12. The turn over frequency (TOF) of the

hybrid  $W_xMo_{1-x}S_2$  materials gradually increases due to presence of both W and Mo atoms, and the activation barrier decreases as shown in the Table S2 and Table S3. Our DFT calculations reveal that the  $MoS_2$  has the lowest TOF among all the systems studied in this work, while  $W_{0.4}Mo_{0.6}S_2$  has the highest.

**Electronic Properties Calculations (Band structures and density of states (DOSs)): the rGO/ $W_{0.4}Mo_{0.6}S_2$  heterostructure.**

The electronic properties calculations (e.g. band and DOSs) were carried out to get a fundamental understanding of the synergistic effects leading to the electrocatalytic activity of the heterostructures formed by rGO with pristine ( $MoS_2$ ,  $WS_2$ ) as well as alloyed materials ( $W_xMo_{1-x}S_2$ , where  $x=0.1 - 0.9$ ) as shown in Figure S11 and Figure 5a. We found that the pristine monolayer  $MoS_2$  and  $WS_2$  are pure semiconductors with high band gap  $\sim 2.5$  eV calculated at B3LYP-D2 level of theory. The calculated lattice constants ( $a$  and  $b$ ) are 2.452 Å, 3.196 Å and 3.176 Å for graphene,  $MoS_2$  and  $WS_2$  respectively. We considered a 4x4 supercell to minimize the lattice mismatch between rGO and the  $W_xMo_{1-x}S_2$  layer. Visualization were performed using VESTA<sup>2</sup> and additional analyses were performed using our in-house codes and scripts.

## Supplementary Figures and Tables

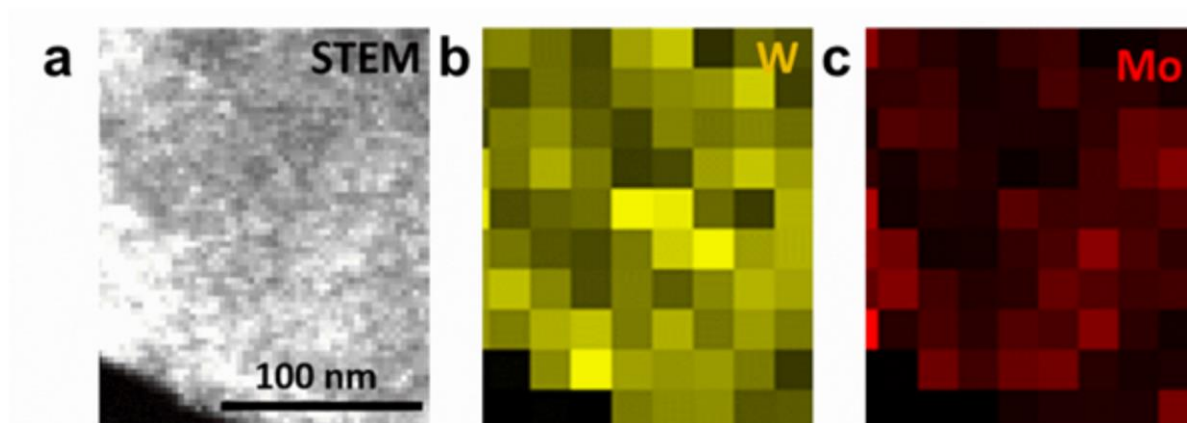

**Figure S1.** (a) STEM image of the rGO/WMoS<sub>2</sub> sample transferred to TEM grid. Elemental mapping by energy dispersive X-ray spectroscopy (EDS) of (b) tungsten (W(M) line); (c) molybdenum (Mo(K) line).

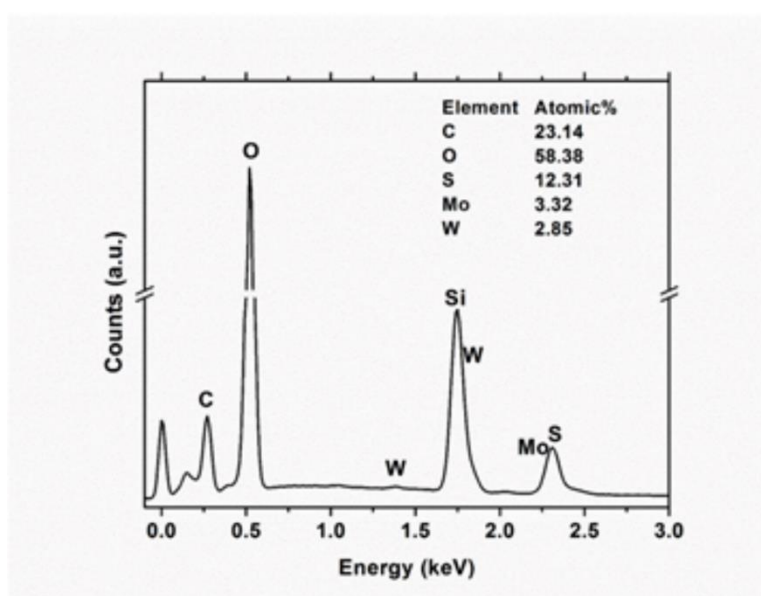

**Figure S2.** EDS spectrum obtained from the rGO/W<sub>x</sub>Mo<sub>1-x</sub>S<sub>2</sub> in Figure 1b, and the atomic ratio between W to Mo is 1:1.16 ( $x=0.46$ ).

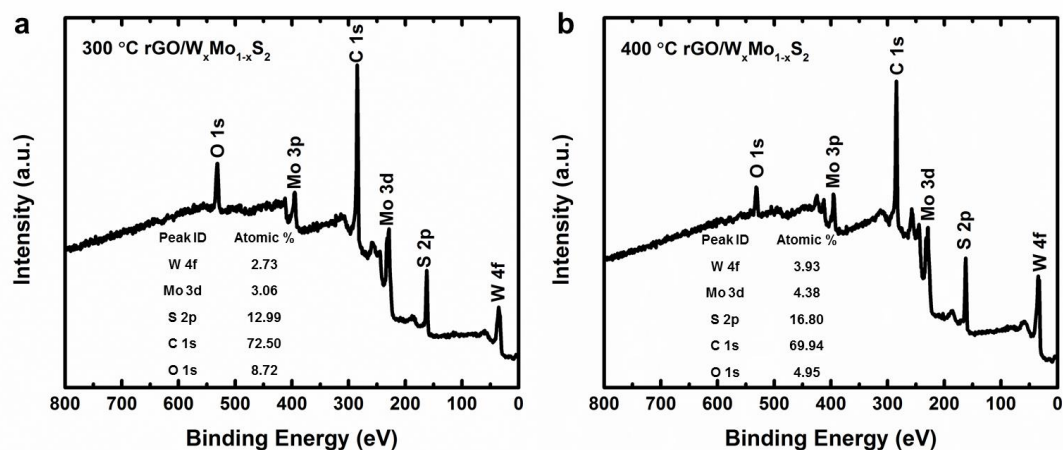

**Figure S3.** XPS survey spectra of rGO/W<sub>x</sub>Mo<sub>1-x</sub>S<sub>2</sub> annealed at (a) 300 °C and (b) 400 °C; the inset tables summarized the elemental composition. Based on the elemental composition, the x values in rGO/W<sub>x</sub>Mo<sub>1-x</sub>S<sub>2</sub> are 0.471 and 0.472 in the sample annealed at 300 and 400 °C, respectively. And the atomic ratio of S:(Mo+W) values are 2.24 and 2.02 in the sample annealed at 300 and 400 °C, respectively.



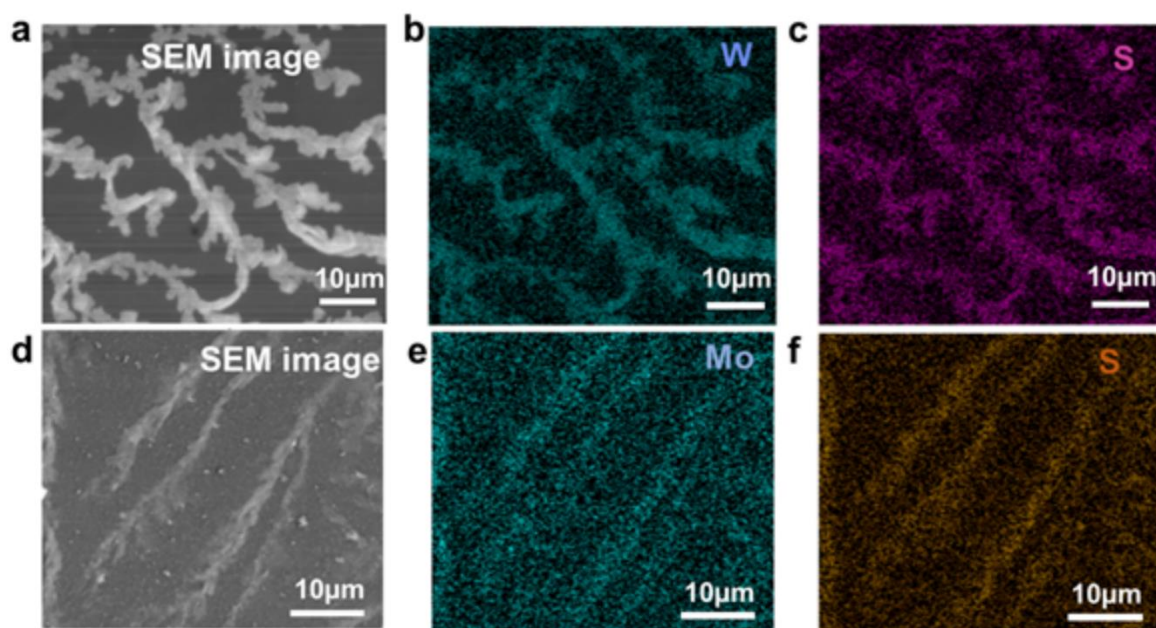

**Figure S4.** (a) SEM image of the rGO/WS<sub>2</sub> sample on a Si/SiO<sub>2</sub> substrate. EDS elemental mappings of: (b) tungsten (W-M line); (c) sulfur (S-K line); (d) SEM image of the rGO/MoS<sub>2</sub> sample on a Si/SiO<sub>2</sub> substrate; EDS mappings of (e) molybdenum (Mo-L line); (f) sulfur (S-K line).

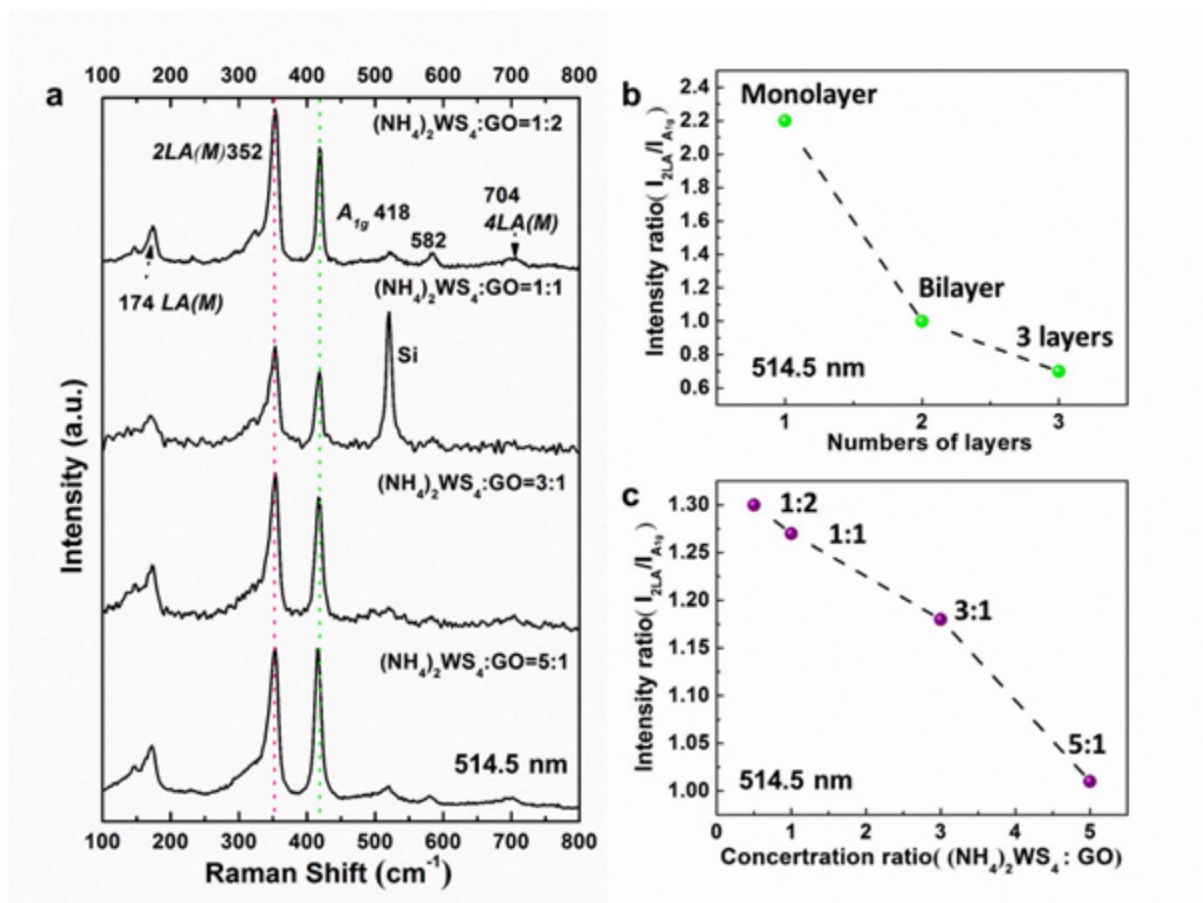

**Figure S5.** (a) Raman spectra of rGO/WS<sub>2</sub> samples with different ratios of (NH<sub>4</sub>)<sub>2</sub>WS<sub>4</sub>/GO used in the precursor; (b) The intensity ratios of  $I_{2LA}/I_{A1g}$  of WS<sub>2</sub> excited by a 514.5 nm laser with the corresponding number of layers,<sup>1</sup> and (c) The intensity ratios of  $I_{2LA}/I_{A1g}$  in rGO/WS<sub>2</sub> samples with different ATTT/GO precursor amounts (excitation 514.5 nm laser).

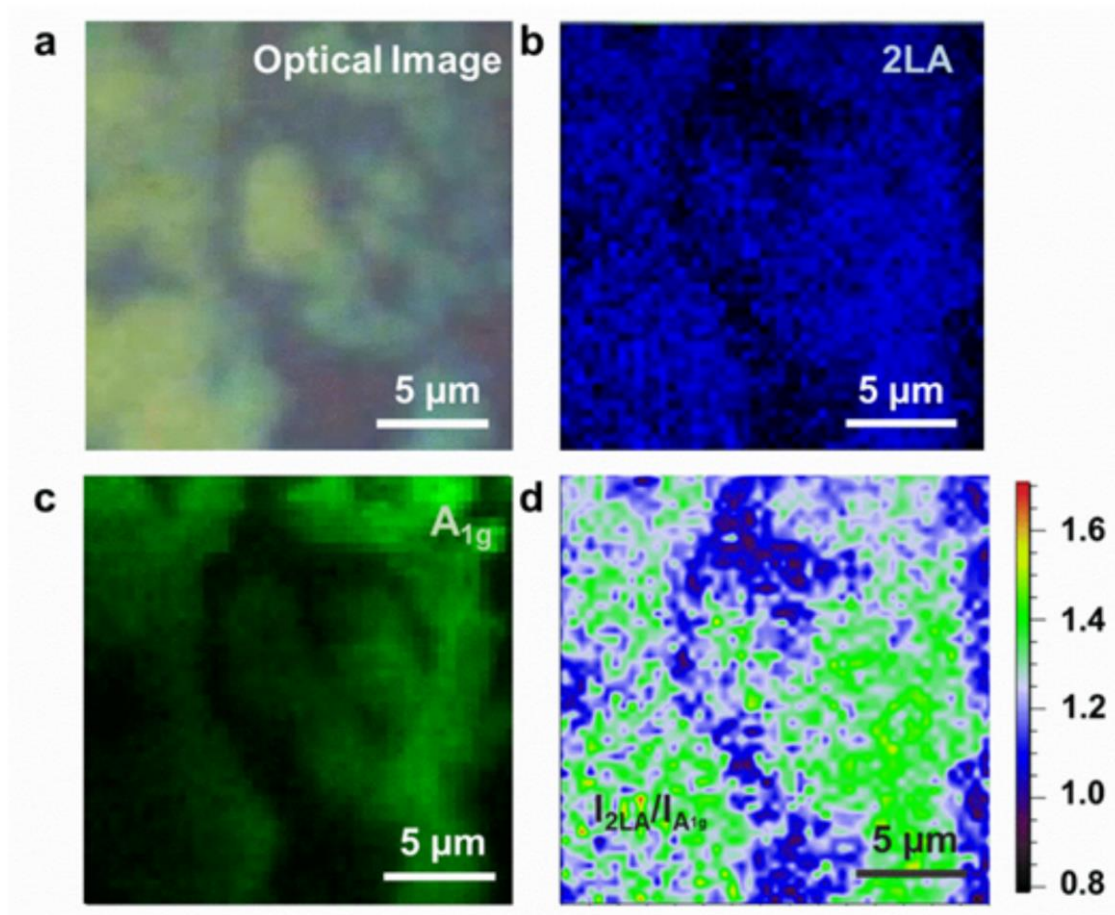

**Figure S6.** Raman mapping characterization of the rGO/WS<sub>2</sub> film. (a) Optical image. (b)  $2LA(M)$  and (c)  $A_{1g}$  intensity maps. (d) Intensity ratio map of  $2LA(M)$  to  $A_{1g}$  modes.

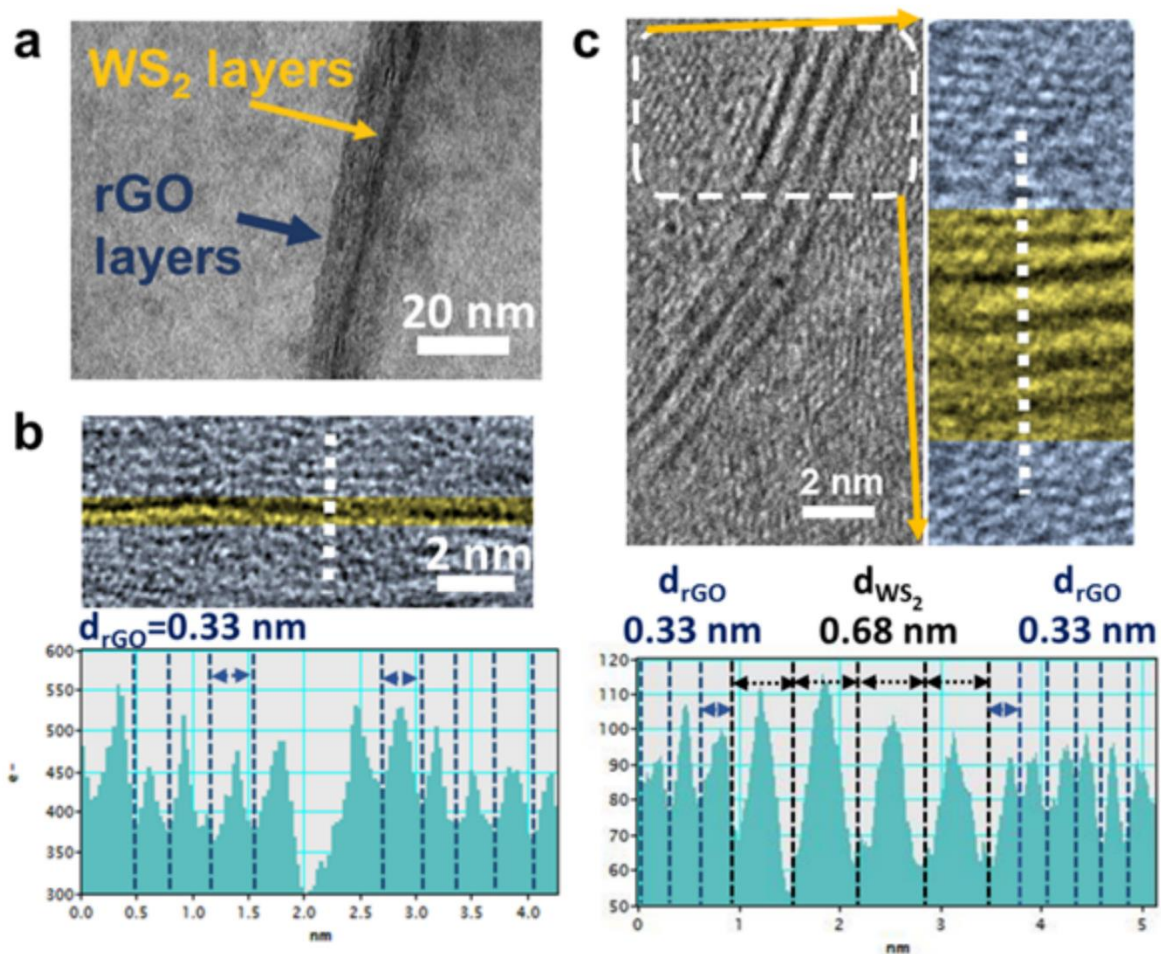

**Figure S7.** (a) TEM image of dendritic-branches of the rGO/WS<sub>2</sub> film; HRTEM image of (b) WS<sub>2</sub> monolayer covered by rGO layer (top panel), and the intensity line profile (bottom panel) of the white dashed line in HRTEM image; and (c) few-layers (top panel) covered by rGO layer, and the intensity line profile (bottom panel) of the white dashed line in HRTEM image. WS<sub>2</sub> layers are marked in yellow and carbon are highlighted in blue.



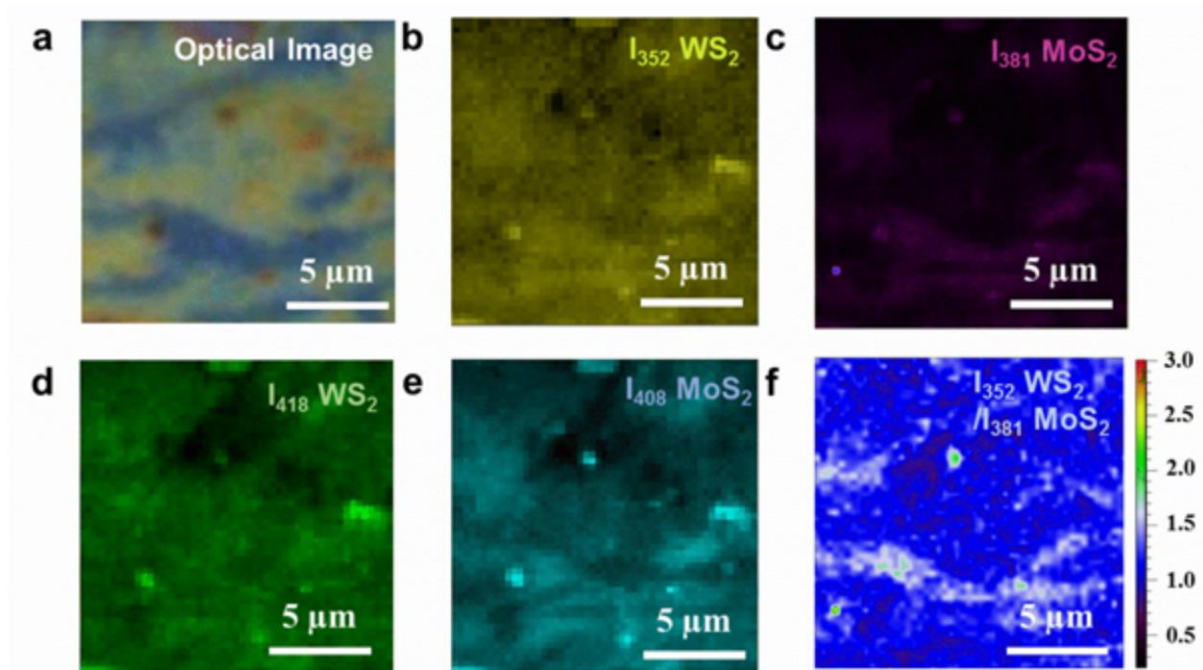

**Figure S8.** (a) Optical image of  $\text{rGO}/\text{W}_x\text{Mo}_{1-x}\text{S}_2$ ; Raman intensity maps of (b)  $\text{WS}_2$  2LA peak ( $352\text{ cm}^{-1}$ ), (c)  $\text{MoS}_2$   $E_{2g}$  peak ( $381\text{ cm}^{-1}$ ), (d)  $\text{WS}_2$   $A_{1g}$  peak ( $418\text{ cm}^{-1}$ ), and (e)  $\text{MoS}_2$   $A_{1g}$  peak ( $408\text{ cm}^{-1}$ ); (f) Intensity ratio map of  $\text{WS}_2$  2LA over  $\text{MoS}_2$   $E_{2g}$ .

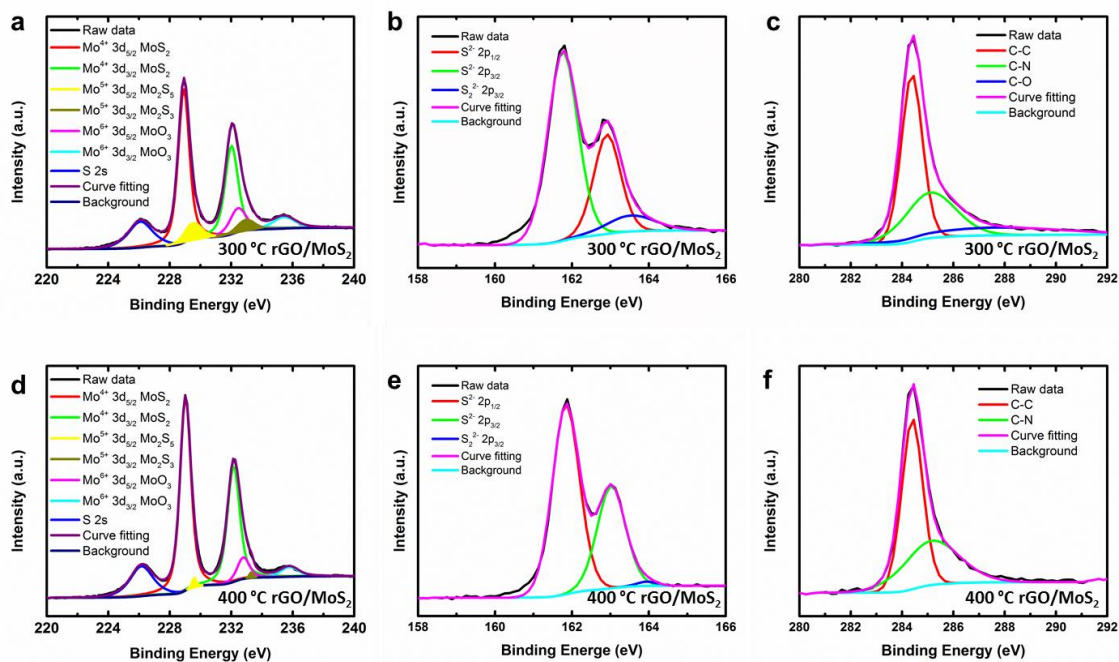

**Figure S9.** High-resolution XPS analysis of (a) Mo 3d, (b) S 2p, and (c) C 1s peaks of rGO/MoS<sub>2</sub> annealed at 300 °C; and the high-resolution XPS analysis of (d) Mo 3d, (e) S 2p, and (f) C 1s peaks of rGO/MoS<sub>2</sub> annealed at 400 °C. The Mo<sup>5+</sup> 3d<sub>5/2</sub> and Mo<sup>5+</sup> 3d<sub>3/2</sub> peaks are filled with yellow and dark yellow color, respectively.

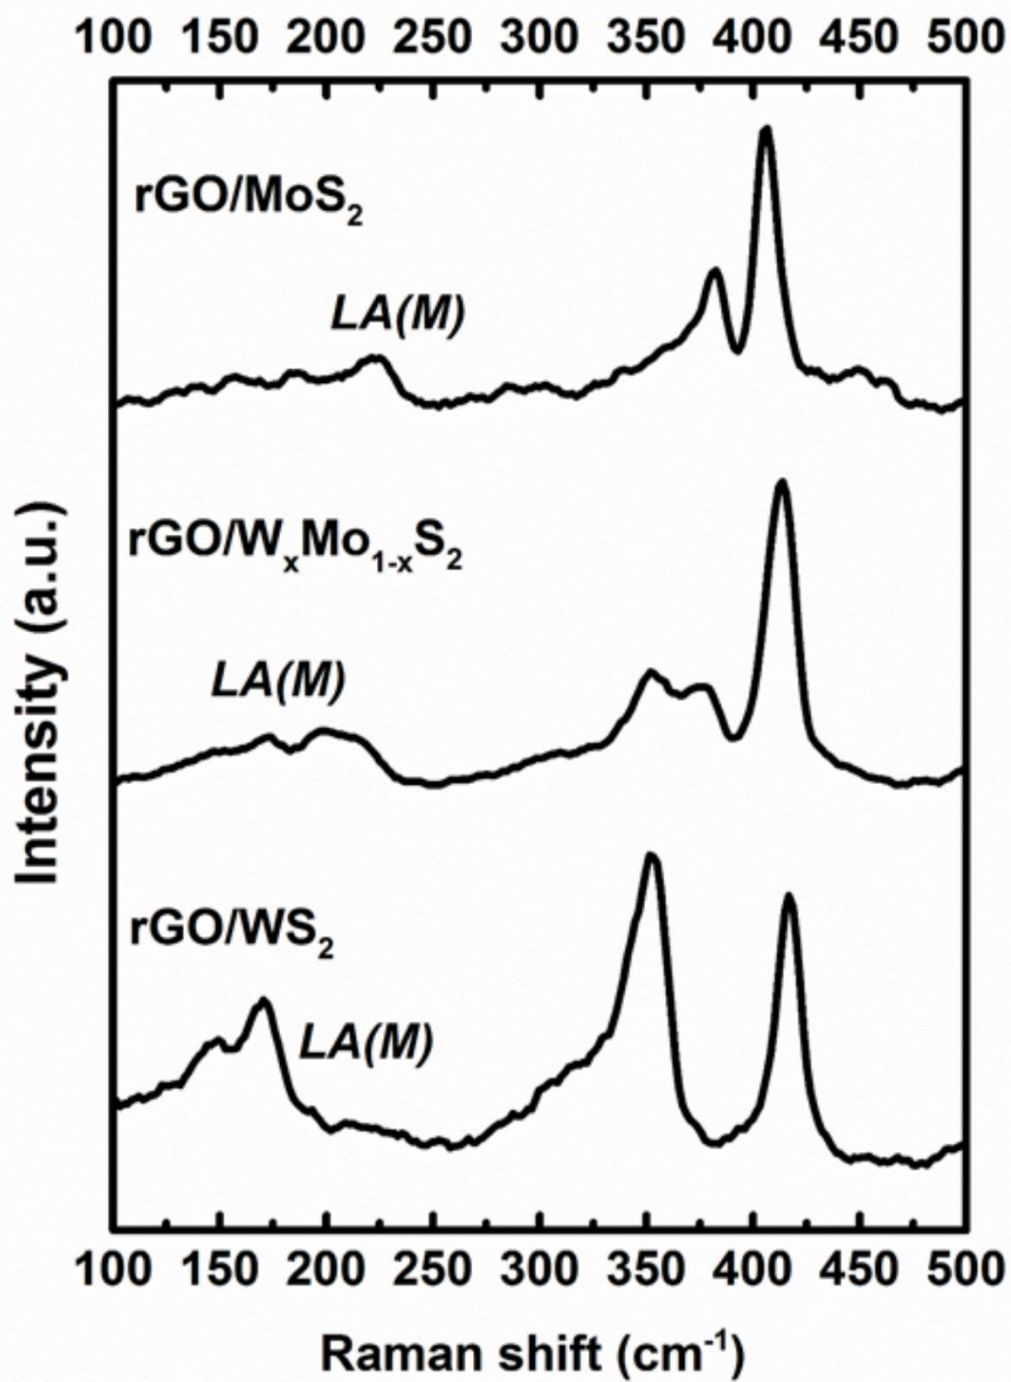

**Figure S10.** Raman spectra of rGO/WS<sub>2</sub>, rGO/W<sub>x</sub>Mo<sub>1-x</sub>S<sub>2</sub>, and rGO/MoS<sub>2</sub> annealed at 300 °C.

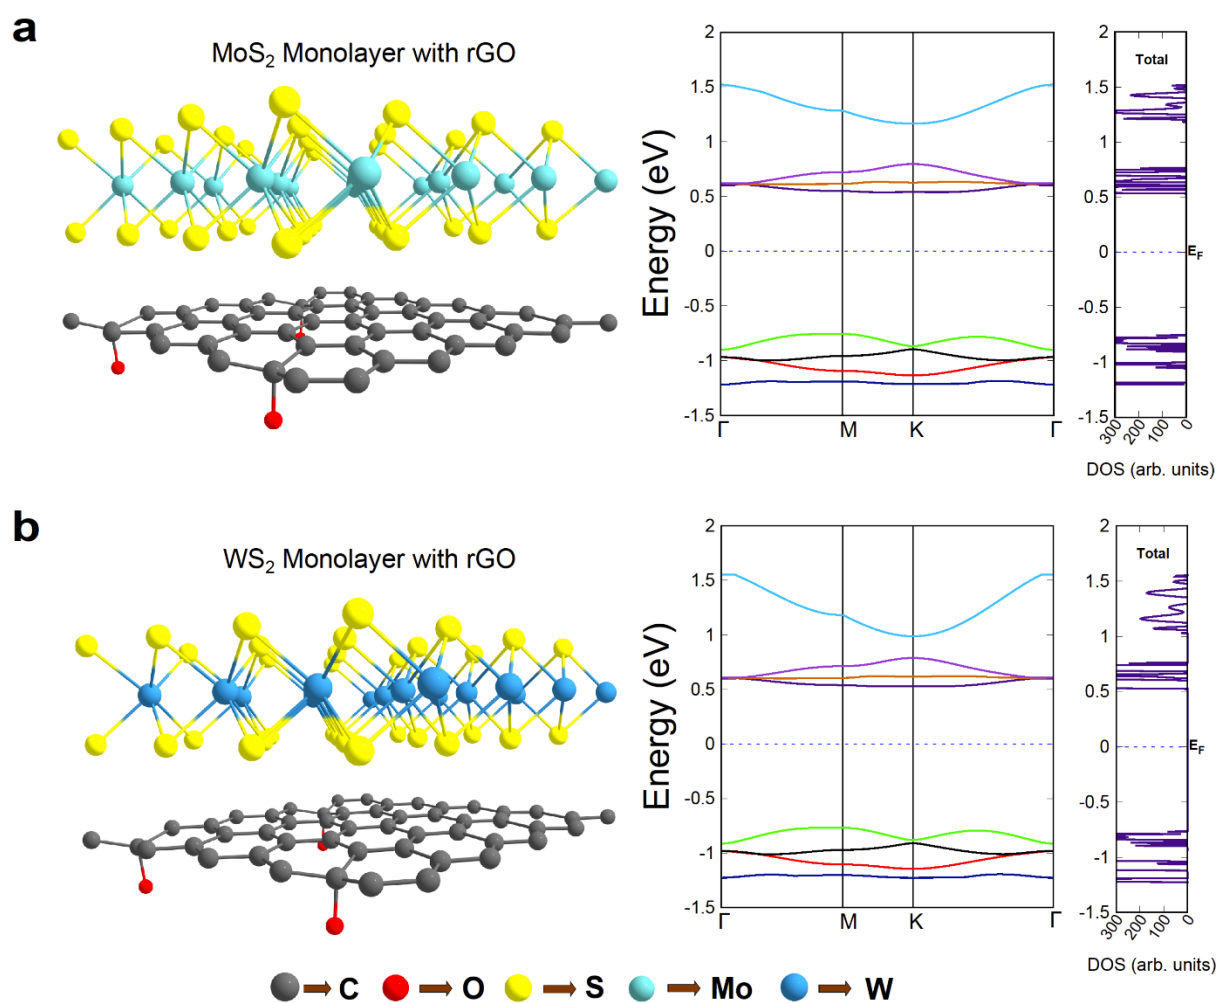

**Figure S11.** Electronic structures, band structures and density of states (DOSs) of the heterostructures formed between rGO and (a) MoS<sub>2</sub> and (b) WS<sub>2</sub>.



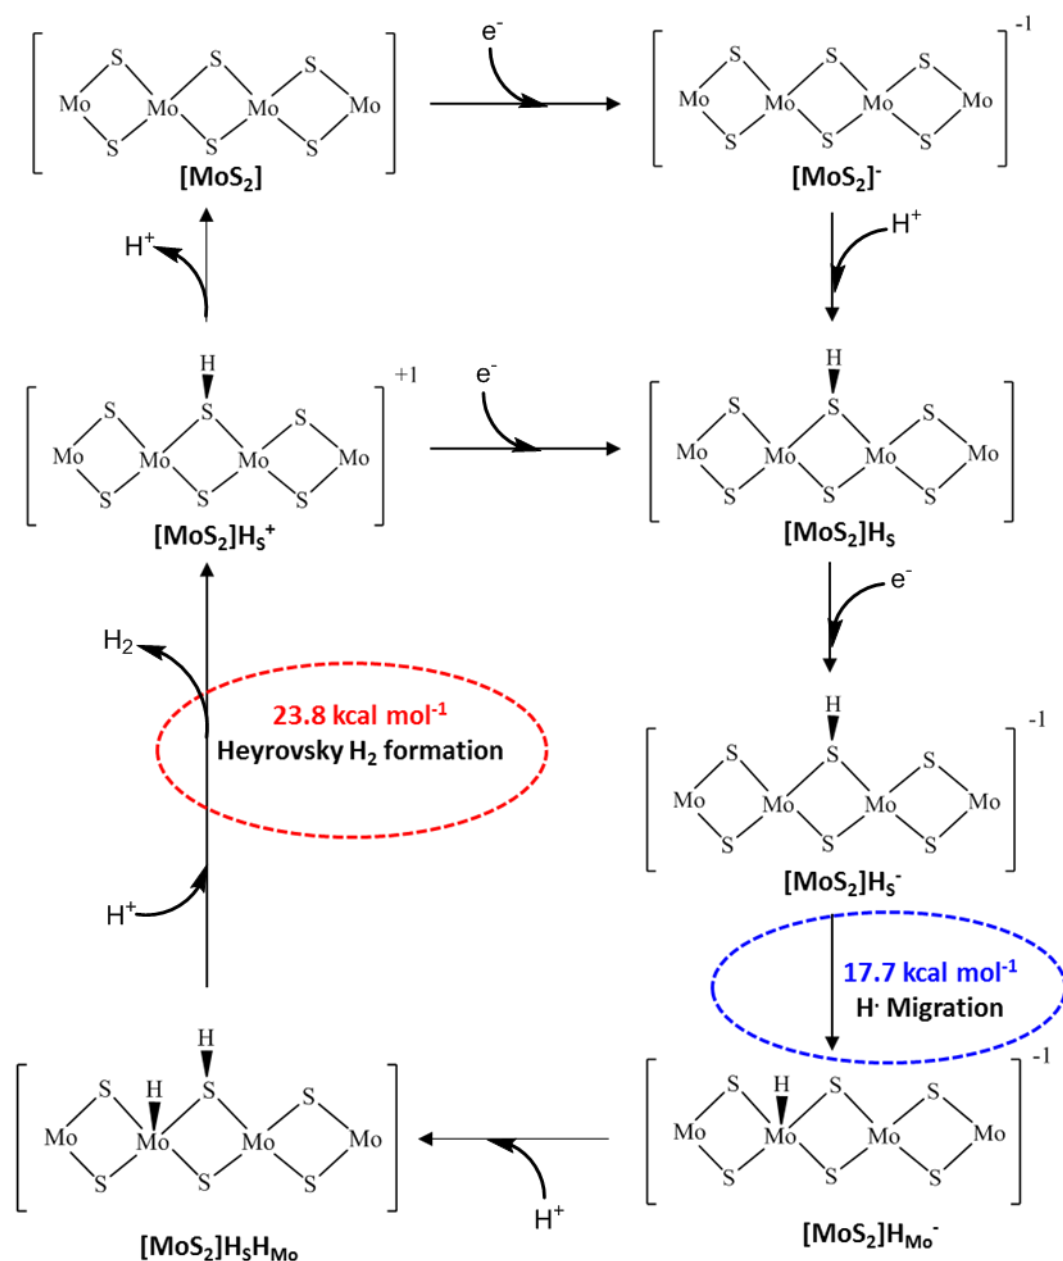

**Figure S12.** Overall chemical reaction mechanism for H<sub>2</sub> evolution on MoS<sub>2</sub> materials using the DFT method with the M06-L functional. M06-L has shown to give accurate energies for reaction barriers involving TMs.<sup>3</sup> The H• migration reaction barrier (Volmer reaction mechanism, highlighted in a dotted blue circle) and the H<sub>2</sub> formation (Heyrovsky reaction mechanism, highlighted in a dotted red circle) on MoS<sub>2</sub> materials are 17.7 kcal mol<sup>-1</sup> and 23.8 kcal mol<sup>-1</sup>, respectively.

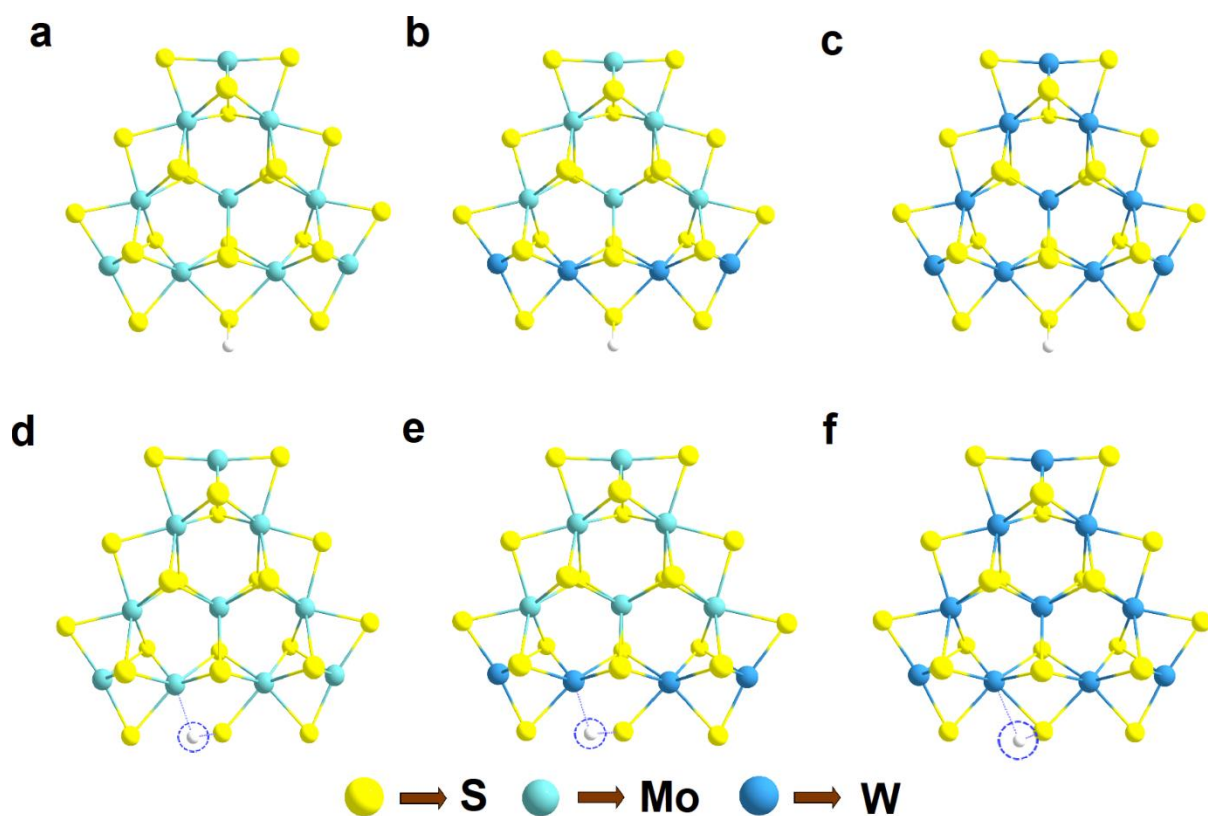

**Figure S13.** The optimized geometries of (a) MoS<sub>2</sub>H<sub>s</sub>, (b) W<sub>x</sub>Mo<sub>1-x</sub>S<sub>2</sub>H<sub>s</sub> (here x=0.4), and (c) WS<sub>2</sub>H<sub>s</sub> materials considered as a model system in the DFT calculations. The transition states (TSs) occurred in the H· migration reaction of these materials are presented in d, e and f, and the position of the H in the TSs is highlighted by a dotted blue circle.

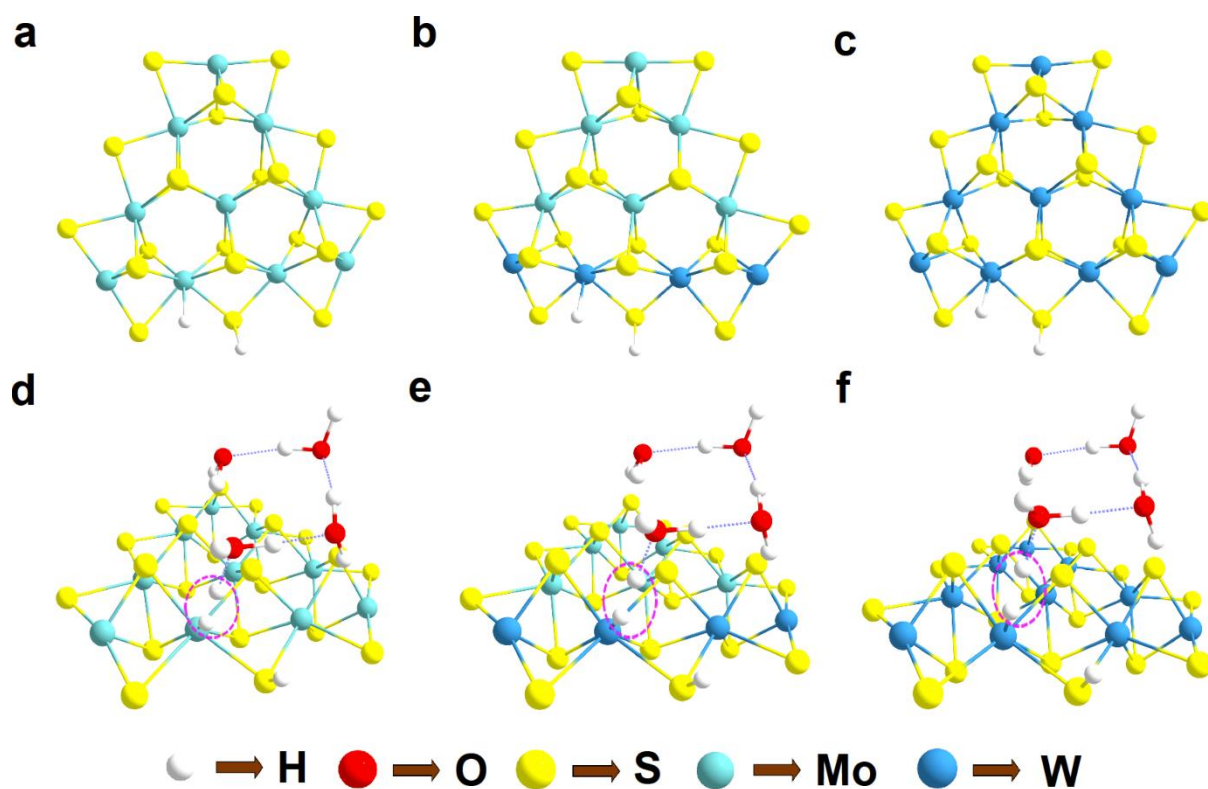

**Figure S14.** The optimized geometries of (a)  $\text{MoS}_2\text{H}_s\text{H}_{\text{Mo}}$ , (b)  $\text{W}_x\text{Mo}_{1-x}\text{S}_2\text{H}_s\text{H}_w$  (here  $x=0.4$ ), and (c)  $\text{WS}_2\text{H}_s\text{H}_w$  materials considered in the DFT calculations. The transition states (TSs) occurred in the Heyrovsky reaction of these materials, TS1, TS2 and TS3 are presented in d, e and f, and the position of the  $\text{H}_2$  in the TSs is highlighted by a dotted pink circle.

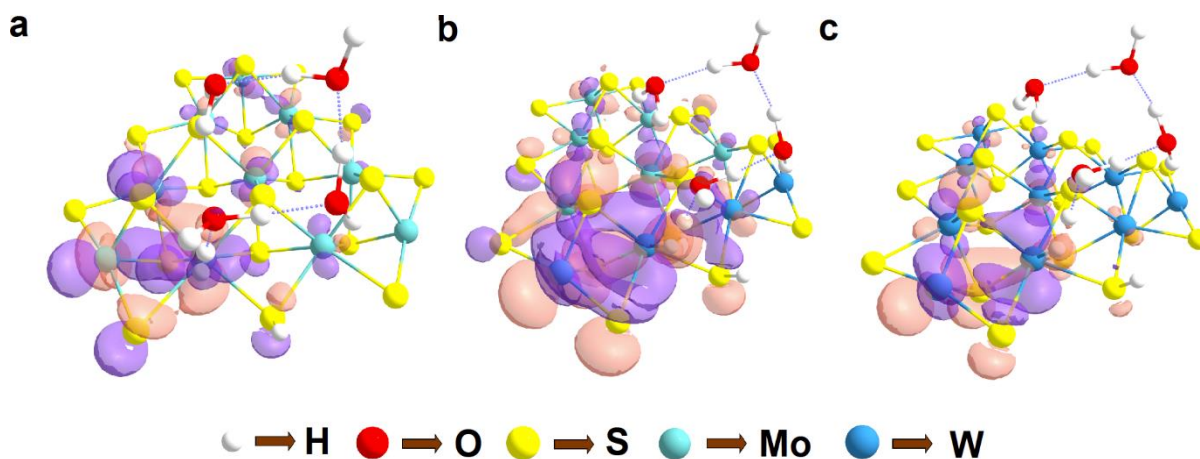

**Figure S15.** Top view of the highest occupied molecular orbital (HOMO) of the transition state structures found in the Heyrovsky reaction mechanism in the presence of four explicit water cluster for: (a) MoS<sub>2</sub> (TS1), (b) W<sub>0.4</sub>Mo<sub>0.6</sub>S<sub>2</sub> (TS2), and (c) WS<sub>2</sub> (TS3). The molecular orbitals involved in the Heyrovsky reaction and activation barrier in HER are highlighted by a dotted pink circle.

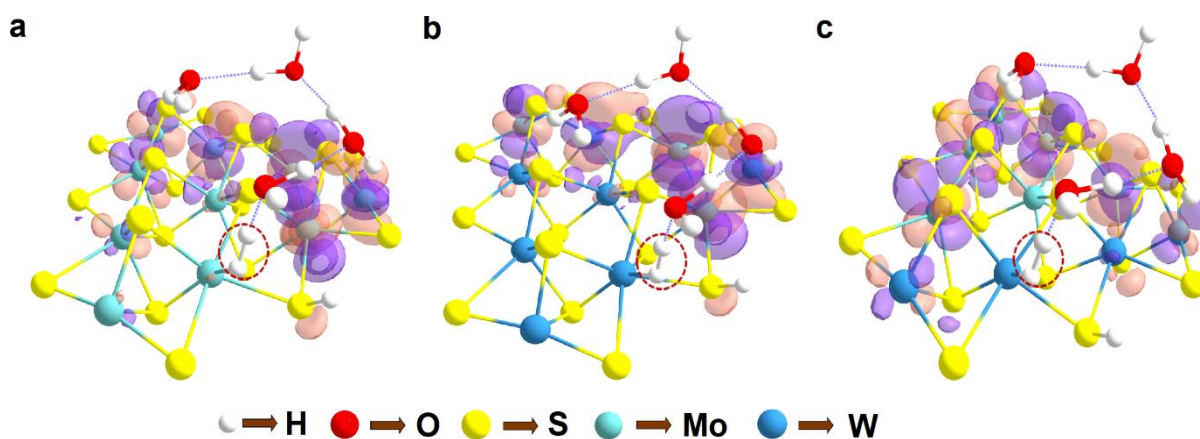

**Figure S16.** Lowest unoccupied molecular orbital (LUMO) of the transition state structures found in the Heyrovsky reaction mechanism in the presence of four explicit water cluster for: (a) MoS<sub>2</sub> (TS1), (b) W<sub>0.4</sub>Mo<sub>0.6</sub>S<sub>2</sub> (TS2), and (c) WS<sub>2</sub> (TS3). The position of the molecular H<sub>2</sub> involved in Heyrovsky reaction are highlighted by a dotted red circle.

**Table S1.** Electrochemical impedance spectroscopy (EIS) fitting and double layer capacitance ( $C_{dl}$ ) calculation results.

| Samples (This work)                                            | $R_p \Omega$ | CPE-T  | CPE-P  | $C_{dl} \text{ mF cm}^{-2}$ |
|----------------------------------------------------------------|--------------|--------|--------|-----------------------------|
| <b>rGO/W<sub>x</sub>Mo<sub>1-x</sub>S<sub>2</sub> (300 °C)</b> | 6.65         | 0.0168 | 0.7903 | 23.39                       |
| <b>rGO/MoS<sub>2</sub> (300 °C)</b>                            | 7.79         | 0.0122 | 0.8253 | 13.25                       |
| <b>rGO/WS<sub>2</sub> (300 °C)</b>                             | 2.69         | 0.0278 | 0.8633 | 37.61                       |
| <b>rGO/W<sub>x</sub>Mo<sub>1-x</sub>S<sub>2</sub> (400 °C)</b> | 5.73         | 0.0177 | 0.7531 | 17.05                       |
| <b>rGO/MoS<sub>2</sub> (400 °C)</b>                            | 4.43         | 0.0252 | 0.7580 | 25.61                       |
| <b>rGO/WS<sub>2</sub> (400 °C)</b>                             | 3.01         | 0.0510 | 0.7925 | 39.29                       |

**Table S2.** H<sup>+</sup> migration reaction energy barriers (Volmer reaction mechanism) obtained for MoS<sub>2</sub>, WS<sub>2</sub>, and hybrid W<sub>x</sub>Mo<sub>1-x</sub>S<sub>2</sub> (x=0.1 – 0.9) materials.

| Compounds                                           | Barrier in kcal mol <sup>-1</sup> | Barrier in kcal mol <sup>-1</sup> |
|-----------------------------------------------------|-----------------------------------|-----------------------------------|
|                                                     | (Gas Phase)                       | (Solvent, water)                  |
| <b>MoS<sub>2</sub></b>                              | 11.9                              | 17.7                              |
| <b>W<sub>0.1</sub>Mo<sub>0.9</sub>S<sub>2</sub></b> | 10.2                              | 14.0                              |
| <b>W<sub>0.2</sub>Mo<sub>0.8</sub>S<sub>2</sub></b> | 09.3                              | 13.9                              |
| <b>W<sub>0.3</sub>Mo<sub>0.7</sub>S<sub>2</sub></b> | 08.0                              | 12.4                              |
| <b>W<sub>0.4</sub>Mo<sub>0.6</sub>S<sub>2</sub></b> | 06.8                              | 11.9                              |
| <b>W<sub>0.5</sub>Mo<sub>0.5</sub>S<sub>2</sub></b> | 08.1                              | 13.0                              |
| <b>W<sub>0.6</sub>Mo<sub>0.4</sub>S<sub>2</sub></b> | 09.6                              | 14.9                              |
| <b>W<sub>0.7</sub>Mo<sub>0.3</sub>S<sub>2</sub></b> | 10.1                              | 12.4                              |

|                                                     |      |      |
|-----------------------------------------------------|------|------|
| <b>W<sub>0.8</sub>Mo<sub>0.2</sub>S<sub>2</sub></b> | 10.7 | 13.1 |
| <b>W<sub>0.9</sub>Mo<sub>0.1</sub>S<sub>2</sub></b> | 11.2 | 15.8 |
| <b>WS<sub>2</sub></b>                               | 12.4 | 18.1 |

**Table S3.** H<sub>2</sub> formation reaction energy barriers (Heyrovsky reaction mechanism) obtained for MoS<sub>2</sub>, WS<sub>2</sub>, and W<sub>x</sub>Mo<sub>1-x</sub>S<sub>2</sub> (x=0.1 – 0.9) with four explicit water molecules and Turnover Frequency (TOF). The unit of TOF is H<sub>2</sub> sec<sup>-1</sup> per edge Mo/W atom.

|                                                     | Barrier in kcal mol <sup>-1</sup> | Barrier in kcal mol <sup>-1</sup> | TOF in sec <sup>-1</sup> |
|-----------------------------------------------------|-----------------------------------|-----------------------------------|--------------------------|
| Compounds                                           | (Gas Phase)                       | (Solvent, water)                  | (Solvent, water)         |
| <b>MoS<sub>2</sub></b>                              | 16.0                              | 23.8                              | 2.1 x 10 <sup>-5</sup>   |
| <b>W<sub>0.1</sub>Mo<sub>0.9</sub>S<sub>2</sub></b> | 13.8                              | 20.1                              | 1.2 x 10 <sup>-2</sup>   |
| <b>W<sub>0.2</sub>Mo<sub>0.8</sub>S<sub>2</sub></b> | 12.5                              | 18.0                              | 4.2 x 10 <sup>-1</sup>   |
| <b>W<sub>0.3</sub>Mo<sub>0.7</sub>S<sub>2</sub></b> | 11.9                              | 15.3                              | 3.5 x 10 <sup>1</sup>    |
| <b>W<sub>0.4</sub>Mo<sub>0.6</sub>S<sub>2</sub></b> | 11.5                              | 13.3                              | 1.1 x 10 <sup>3</sup>    |
| <b>W<sub>0.5</sub>Mo<sub>0.5</sub>S<sub>2</sub></b> | 12.2                              | 14.0                              | 3.3 x 10 <sup>2</sup>    |
| <b>W<sub>0.6</sub>Mo<sub>0.4</sub>S<sub>2</sub></b> | 13.0                              | 15.1                              | 5.1 x 10 <sup>1</sup>    |
| <b>W<sub>0.7</sub>Mo<sub>0.3</sub>S<sub>2</sub></b> | 13.3                              | 17.1                              | 1.9 x 10 <sup>0</sup>    |
| <b>W<sub>0.8</sub>Mo<sub>0.2</sub>S<sub>2</sub></b> | 13.5                              | 18.4                              | 2.1 x 10 <sup>-1</sup>   |
| <b>W<sub>0.9</sub>Mo<sub>0.1</sub>S<sub>2</sub></b> | 14.0                              | 19.8                              | 1.7 x 10 <sup>-2</sup>   |
| <b>WS<sub>2</sub></b>                               | 14.5                              | 21.3                              | 1.5 x 10 <sup>-3</sup>   |

## References

- (1) Berkdemir, A.; Gutiérrez, H. R.; Botello-Méndez, A. R.; Perea-López, N.; Elías, A. L.; Chia, C.-I.; Wang, B.; Crespi, V. H.; López-Urías, F.; Charlier, J.-C. Identification of Individual and Few Layers of WS<sub>2</sub> Using Raman Spectroscopy. *Sci. Rep.* **2013**, *3*.
- (2) Momma, K.; Izumi, F. VESTA 3 for Three-Dimensional Visualization of Crystal, Volumetric and Morphology Data. *J. Appl. Crystallogr.* **2011**, *44*, 1272–1276.
- (3) Huang, Y.; Nielsen, R. J.; Goddard III, W. A.; Soriaga, M. P. The Reaction Mechanism with Free Energy Barriers for Electrochemical Dihydrogen Evolution on MoS<sub>2</sub>. *J. Am. Chem. Soc.* **2015**, *137*, 6692–6698.
